# Supplementary material for: Integrability of a globally coupled complex Riccati array: quadratic integrate-and-fire neurons, phase oscillators and all in between
Source: arXiv:2305.17683 ancillary file (2024-02-07)
Supplement: Supplementary file 1 [file supplemental.pdf]

# Supplemental Material

Integrability of a globally coupled complex Riccati array: quadratic integrate-and-fire neurons, phase oscillators and all in between

Rok Cestnik* and Erik A. Martens

## MAIN RESULT SUMMARY

Complex Riccati arrays $x_j(t) \in \mathbb{C}$, $j = 1, ..., N$:

$$\dot{x}_j = a x_j^2 + b x_j + c \,, \tag{S1}$$

subject to global forcing functions $a(t), b(t), c(t) \in \mathbb{C}$ are exactly described by the Möbius transformation:

$$x_j = Q + \frac{y\,\xi_j}{1 + s\,\xi_j} \,, \tag{S2}$$

where complex variables $Q, y, s \in \mathbb{C}$ evolve according to:

$$\dot{Q} = aQ^2 + bQ + c \,, \tag{S3a}$$
$$\dot{y} = (b + 2aQ)y \,, \tag{S3b}$$
$$\dot{s} = -ay \,, \tag{S3c}$$

and $\xi_j$ are constants determined by initial values of $x_j$. Thus, the six-dimensional system (S3) represents a low dimensional reductions of the $2N$-dimensional complex valued Riccati array (S1) in terms of the macroscopic variables $Q, y, s$.

## PROOF OF THE MAIN RESULT

The main result can be proven in just a few lines as follows. Taking the derivative of the transformation (S2) with respect to time,

$$\dot{x}_j = \dot{Q} + \dot{y}\frac{\xi_j}{1 + s\xi_j} - \dot{s}y\left(\frac{\xi_j}{1 + s\xi_j}\right)^2,$$

and substituting (S1) and (S3) into left and right hand sides respectively, we obtain

$$ax_j^2 + bx_j + c = aQ^2 + bQ + c + \frac{(b + 2aQ)y\xi_j}{1 + s\xi_j} + a\left(\frac{y\xi_j}{1 + s\xi_j}\right)^2.$$

The two terms $c$ trivially cancel on both sides, and the terms proportional to $b$ cancel due to (S2). Eliminating the common factor $a$ in the remaining terms, we have

$$x_j^2 = Q^2 + 2Qy\frac{\xi_j}{1 + s\xi_j} + \left(y\frac{\xi_j}{1 + s\xi_j}\right)^2,$$

which is nothing but the square of relation (S2). This proves that dynamics (S1) and (S3) are equivalent.

## INITIAL CONSTRAINTS

Transformation (S2) can be easily inverted:

$$\xi_j = \frac{x_j - Q}{y - s(x_j - Q)} \,. \tag{S4}$$

This helps us choose the desired relation between constants of motion $\xi_j$ and initial conditions of both system variables $x_j(0)$ and dynamical variables $Q(0), y(0), s(0)$.

For the relation between $\xi_j$ and $x_j(0)$ to be identical we set $Q(0) = s(0), y(0) = 1$ which we refer to as "identity conversion" in the main text. In some cases an "improper" choice of initial conditions can lead the macroscopic variables $Q, y, s$ to diverge. Such is the case if we choose the "identity conversion" when $a, b, c \in \mathbb{R}$ and $x_j \in \mathbb{R}$ – as a result, $Q(t)$ in Eq. (S3) can be shown to diverge. This divergence can be avoided by a suitable choice of initial conditions. For example, choosing $Q(0) = \mathrm{i}$ resolves the divergence issue. For the other two variables we set $y(0) = -2\mathrm{i}, s(0) = 1$ so that expression (S4) simplifies: $\xi_j = \frac{\mathrm{i} - x_j(0)}{\mathrm{i} + x_j(0)} = e^{\mathrm{i}\,2\,\mathrm{atan}(x_j(0))}$. We refer to this initial constraint as "Möbius conversion" in the main text.

Various other initial constraints could be useful in different systems, for example $\sum_j \xi_j = 0$, cf. (4.12) in [1]. This can be achieved by setting $Q(0) = \langle x_j(0) \rangle$, $y(0) = 1$, $s(0) = 0$. The constants then express as $\xi_j = x_j(0) - \langle x_j(0) \rangle$, where $\langle \cdot \rangle$ represents the ensemble average. In the particular case of phase oscillators in the thermodynamic limit this constraint is convenient in explaining the link between Watanabe-Strogatz theory [2] and the Ott-Antonsen ansatz [3]: if the phases (i.e., the arguments of $x_j$) are distributed according to a wrapped Cauchy-Lorentz distribution, then $Q$ is equivalent to the Kuramoto order parameter and the constants of motion do not contribute to the evolution of the macroscopic state (cf. Section 2.3 in [4]).

## CONNECTION TO THE WATANABE-STROGATZ THEORY

The Watanabe-Strogatz theory [1, 2, 5] (WS) considers phase oscillators with global sinusoidal coupling:

$$\dot{\varphi}_j = \omega + 2\,\mathrm{Im}[he^{-i\varphi_j}] = \omega - i(he^{-i\varphi_j} - \bar{h}e^{i\varphi_j}) \,, \tag{S5}$$

where $\omega(t) \in \mathbb{R}$ is a real-valued instantaneous frequency and $h(t) \in \mathbb{C}$ any complex forcing. The theory provides a

low dimensional description, showing that the evolution of phases $\varphi_j$ can be described by a Möbius transform of 3 global dynamical variables and constants $\psi_j$ determined by initial conditions. Here we show that this is a particular case of transformation (S2) and equations (S3) under conditions:

$$a = -\bar{c}\,, \quad \mathrm{Re}[b] = 0\,, \quad |x_j| = 1\,, \tag{S6}$$

which with identity conversion (4) imply the constraint:

$$s = \bar{Q}(Qs + y)\,, \tag{S7}$$

(cf. Eq. (39) in [6]). Let us express the phase dynamics Eqs. (S5) using a complex-valued exponential $x_j = e^{\mathrm{i}\varphi_j}$:

$$\dot{x}_j = -\bar{h}x_j^2 + \mathrm{i}\omega x_j + h\,, \tag{S8}$$

to see how this is a special case of the general complex Riccati equation (S1) with $c = -\bar{a} = h$ and $b = \mathrm{i}\omega$. Now let us write the dynamics of the quantity: $Y = Qs + y$ under conditions (S6):

$$\dot{Y} = (aQ + b - \bar{a}\bar{Q})Y\,. \tag{S9}$$

Notice how the quantity $aQ + b - \bar{a}\bar{Q}$ is purely imaginary, which (using the identity conversion (4): $Y(0) = 1$) implies that $Y$ is fully determined by its complex angle, $\theta \in \mathbb{R}$, $Y = e^{\mathrm{i}\theta}$, evolving according to

$$\dot{\theta} = |b| + 2\mathrm{Im}[aQ] = \omega - \mathrm{i}(h\bar{Q} - \bar{h}Q)\,. \tag{S10}$$

We identify Eq. (S10) as the WS angle equation, cf. Eq. (23b) in [5]. Together with Eq. (S3a) they form the complete WS description of the dynamics for system (S5), cf. Eq. (23a) in [5] [7]. One can check that Eq. (S3c) for $s$, under conditions (S6) also yields (S10).

Thus, our formalism reproduces the WS theory for the special case (S6). The phases $\varphi_j$ are simply complex arguments of variables $x_j = e^{\mathrm{i}\varphi_j}$ and the WS constants of motion $\psi_j$ are complex arguments of constants $\xi_j = e^{\mathrm{i}\psi_j}$ if "identity conversion" (4) is used.

## CYCLES IN THE COMPLEX QIF MODEL

Consider the QIF model without coupling ($\epsilon = 0$). While the real QIF model cannot exhibit any limit cycles due to its low dimensionality, cyclic orbits may in principle occur in the complex QIF model; their existence can be shown as follows. The complex QIF model:

$$\dot{x} = x^2 + I, \tag{S11}$$

can be rewritten in terms of $x = v + iw$ with $v, w \in \mathbb{R}$,

$$\dot{v} = v^2 - w^2 + I, \tag{S12}$$

$$\dot{w} = 2vw. \tag{S13}$$

It is easy to see that for $I < 0$, this system has an attractor and repeller ($w = 0$ with $v = \pm\sqrt{I}$), while for $I > 0$ there are two centers at $v = 0$ with $w = \pm\sqrt{I}$. Furthermore, (S11) has a time reversal symmetry, i.e., it is invariant to the involution $v \mapsto -v$, $t \mapsto -t$. According to a theorem of nonlinear centers for reversible systems (see, e.g., [8]) this symmetry guarantees the existence of closed orbits close to the center for $I > 0$ .

## THERMODYNAMIC LIMIT

Our formalism works for any number of units $N$, even in the thermodynamic limit $N \to \infty$ where the variables $Q, y, s$ describe the macroscopic state in terms of average quantities, e.g., $\langle x_j \rangle = Q + \sum_{n=1}^{\infty}(-s)^{n-1}\langle \xi_j^n \rangle$. Since $\xi_j$ are constant, the sum represents a function of $s$ that does not change in time (denoted in [9, 10] as $\mathcal{M}(s)$). If we consider the known special cases of phase oscillators or QIF neurons, then $\langle x_j \rangle$ represents the Kuramoto order parameter or the mean voltage respectively. If additionally the distribution of phases $\varphi_j = \arg(x_j)$ is a wrapped Cauchy-Lorentzian (or for QIF if $x_j$ are Cauchy-Lorentzian), then choosing constants according to $\xi_j = x_j(0) - \langle x_j(0) \rangle$ yields all the constants' moments zero [4]: $\langle \xi_j^n \rangle = 0$, and thus the complete ensemble is described by a single complex order parameter: $\langle x_j^n \rangle = Q^n$, evolving according to Eq. (S3a). This corresponds to the Ott-Antonsen ansatz for phase oscillators [3] and the Lorentzian ansatz for QIF neurons [11]. For the general case $a, b, c, x_j \in \mathbb{C}$ there are likely further ways in which particular initial conditions lead to an additional dynamical reduction, but we leave this investigation for future work.

## ADDITIONAL EXAMPLE IV:

*Thermodynamic limit and integral simplifications.* Previously, the thermodynamic limit of pure phase oscillators subject to noise or frequency inhomogeneities were considered [6]. In certain cases, such oscillators behave just like having the addition of a complex frequency component and thus, the six dimensional generalization (S3) can be used. Here we start with the complex oscillators and ask how do the dynamics look in the continuum limit of infinite ensembles, $N \to \infty$. We can express the sum in the generalized Kuramoto order parameter (11) as an integral,

$$Z_1 = Q + y \int \frac{\xi}{1 + s\xi}\mathrm{d}\xi\,. \tag{S14}$$

Can this integral be simplified for certain initial conditions? Consider as an example the special case of initial states where the oscillators start uniformly distributed on a circle with center $q$ and amplitude $\rho$, i.e., $\xi = q + \rho e^{\mathrm{i}\phi}$

(using the identity conversion (4)). Then the integral can be performed over the angle $\phi$,

$$\int \frac{\xi}{1+s\xi}\mathrm{d}\xi = \frac{1}{2\pi}\int_0^{2\pi} \frac{q+\rho e^{\mathrm{i}\phi}}{1+qs+\rho s e^{\mathrm{i}\phi}}\mathrm{d}\phi = \frac{q}{1+qs}\,, \tag{S15}$$

and so in this case the order parameter $Z_1$ can be expressed as

$$Z_1 = Q + \frac{qy}{1+qs}\,. \tag{S16}$$

Notice that the radius of the circle $\rho$ is insignificant – therefore, the expression (S16) also applies to homogeneous initial conditions on a disk or an annulus. One can expect that more general initial conditions (such as a wrapped Cauchy distribution on a ring) can also be simplified in a similar way, but this is a subject for future research.

Let us consider the system (16) again with a continuum of oscillators initially distributed uniformly on a circle around $q = 0.3 + 0.3\mathrm{i}$ with radius $\rho = 0.5$ (the radius does not matter). Since we can express $Z_1$ explicitly with $Q, y, s$ variables (S16), we have a closed system of equations,

$$\begin{aligned}\dot{Q} &= 0.75Q^2 - 0.75 + \left(\mathrm{i} - 0.7\mathrm{i}\ \mathrm{Im}\left[Q + \frac{qy}{1+qs}\right]\right)Q\,,\\ \dot{y} &= 1.5Qy + \left(\mathrm{i} - 0.7\mathrm{i}\ \mathrm{Im}\left[Q + \frac{qy}{1+qs}\right]\right)y\,,\\ \dot{s} &= -0.75y\,.\end{aligned} \tag{S17}$$

We simulate the reduced system (S17) and compare it to a discretized one with $N = 1000$ oscillators. The resulting trajectories overlap, as shown in Fig. S1. Remarkably, the order parameter $Z_1(t)$ is perfectly periodic, while individual oscillators are chaotic.

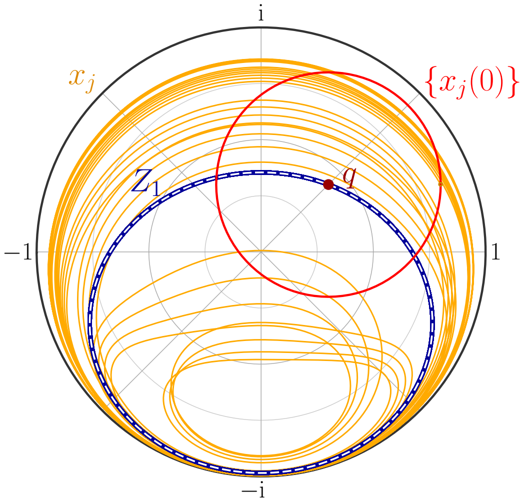


FIG. S1. Continuum limit ($N \to \infty$) of the complex generalization of Josephson junction array (16). The initial conditions are uniformly distributed on a circle around $q = 0.3+0.3\mathrm{i}$ depicted in red. Such special initial conditions allow for an exact solution since the expression for $Z_1$ can be analytically solved, see (S16). A single trajectory depicted in orange, exhibiting chaotic motion. The trajectory of the generalized Kuramoto order parameter $Z_1$ (11) depicted in blue is perfectly periodic, and overlaid in dotted white is the finite simulation with $N = 1000$ for comparison (they are indistinguishable).

* rok.cestnik@math.lth.se


[1] S. Watanabe and S. H. Strogatz, Physica D **74**, 197 (1994).
[2] S. Watanabe and S. H. Strogatz, Phys. Rev. Lett. **70**, 2391 (1993).
[3] E. Ott and T. M. Antonsen, Chaos **18**, 037113 (2008).
[4] A. Pikovsky and M. Rosenblum, Physica D **240**, 872 (2011).
[5] S. A. Marvel, R. E. Mirollo, and S. H. Strogatz, Chaos **19**, 043104 (2009).
[6] R. Cestnik and A. Pikovsky, Chaos **32**, 113126 (2022).
[7] Note that in [5] they consider the complex conjugate of the quantity $Q$, which they denote by $\alpha$.
[8] S. H. Strogatz, *Nonlinear dynamics and chaos with student solutions manual: With applications to physics, biology, chemistry, and engineering* (CRC press, 2018).
[9] R. Cestnik and A. Pikovsky, Phys. Rev. Lett. **128**, 054101 (2022).
[10] B. Pietras, R. Cestnik, and A. Pikovsky, Phys. Rev. E **107**, 024315 (2023).
[11] E. Montbrió, D. Pazó, and A. Roxin, Physical Review X **5**, 021028 (2015), 1506.06581.
